# Supplementary material for: ME-Brain-1.0: Memory, Cognition and Action for Evolving Embodied Intelligence
Source: arXiv:2609.24271 source file (2026-09-29)
Supplement: Supplementary file 1 [file A_appendix.tex]

%% sec/A_appendix.tex

\section{Acceleration of the Infra Operator}
\label{app:infra_accel}

Section~\ref{sec:infra:accel} describes the fused operator leveraged during training for
acceleration, which is designed for the MoE MLP module to reduce the communication and
computation overhead. The end-to-end acceleration effects of the operator on the
Qwen3.5 35B A3B model are shown under different parallel parameter configurations.
When configured with \texttt{tp=8, ep=8}, the operator accelerates by 2\%
(656\,s/step $\to$ 642\,s/step); when configured with \texttt{tp=8, ep=4}, the
operator accelerates by 17\% (681\,s/step $\to$ 580\,s/step). This indicates that the
lower the proportion of communication time, the more pronounced the overall acceleration
effect of the operator.

\section{Derivation of the MOPD Objective}
\label{app:mopd_deriv}

Section~\ref{sec:pt:mopd} (Eq.~\ref{eq:mopd}) writes the MOPD loss as a routed mixture
of token-level reverse-KL divergences under the student's on-policy distribution. This
appendix records the three quantities deferred for brevity: the single-sample estimator
we use in place of the exact reverse KL, the magnitude-preserving diagnostic we log for
monitoring, and the clipped policy-gradient surrogate we actually back-propagate.

\parab{(a) Single-sample $k_1$ estimator of the reverse KL.}
For a single realised token $y_t \sim \pi_\theta(\cdot\mid x, y_{<t})$, Schulman's
low-variance $k_1$ estimator of the per-token reverse KL is:
\begin{equation}
  \widehat{D}_{\mathrm{KL}}^{k_1}\!\bigl(\pi_\theta \,\|\, \pi_{T_k}\bigr)_t
  = \log\pi_\theta(y_t \mid x, y_{<t}) - \log\pi_{T_k}(y_t \mid x, y_{<t})
  \label{eq:k1}
\end{equation}

\parab{(b) Magnitude-preserving diagnostic $\mathcal{L}_{\mathrm{abs}}$.}
Because the $k_1$ estimator is signed, its running average can hover near zero even when
the token-level teacher$\|$student gap is large. We therefore log alongside the signed
loss a magnitude-preserving diagnostic:
\begin{equation}
  \mathcal{L}_{\mathrm{abs}}(\theta) = \mathbb{E}\!\left[\frac{1}{|y|}\sum_{t=1}^{|y|}
  \Bigl|\log\pi_\theta(y_t\mid x,y_{<t}) - \log\pi_{T_k}(y_t\mid x,y_{<t})\Bigr|\right]
  \label{eq:labs}
\end{equation}

\parab{(c) Clipped policy-gradient surrogate $\mathcal{L}_{\mathrm{distill}}$.}
Because rollouts are produced asynchronously by an inference engine at parameters
$\theta_{\mathrm{old}}$ while the training engine has since advanced to $\theta$,
samples are strictly off-policy at the moment of the gradient step. We treat the negated
$k_1$ estimator as a per-token advantage and optimize the clipped surrogate with
$\epsilon = 0.2$.

\section{Ablations on the Reasoning Expert in MOPD}
\label{app:mopd_ablations}

Before scaling MOPD to the full production run, we ran a progressive teacher-composition
study in which teachers were added one domain at a time. The purpose was not merely to
select a final recipe, but to expose \emph{cross-domain transfer effects} (both synergies
and conflicts) between task-specific experts.

The clearest illustration comes from a pair that differs by a single teacher: one
configuration distills from tool-use, IF, and safety teachers; the other extends it with
a code teacher, holding every other component fixed. Adding the code teacher produces
the following observations: Reasoning-oriented benchmarks improve substantially
(LCB-V6 by $+3.81$, AIME25 by $+2.30$, AIME26 by $+0.83$). Non-reasoning axes also
improve: Content-SafetyBench by $+0.85$, Behavioral-SafetyBench by $+4.06$, IFEval by
$+2.14$, and IFBench by $+0.55$. These results confirm that code is a first-class domain
in every subsequent MOPD configuration, and that every capability the practitioner
intends to preserve or improve should be represented by at least one teacher in the joint
distillation.
